# Supplementary material for: StreamingT2V: Consistent, Dynamic, and Extendable Long Video Generation from Text
Source: arXiv:2403.14773 source file (2025-04-16)
Supplement: Supplementary file 2 [file our-all-2.tex]

\begin{subfigure}{\textwidth}
    \hspace*{\fill}
    
    \includegraphics[width=0.11\textwidth]{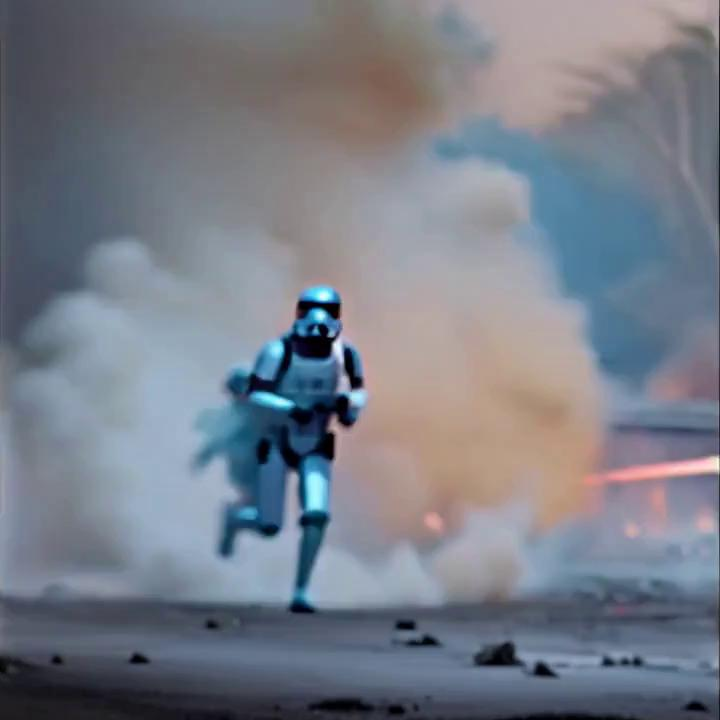}
    \hfill
    \includegraphics[width=0.11\textwidth]{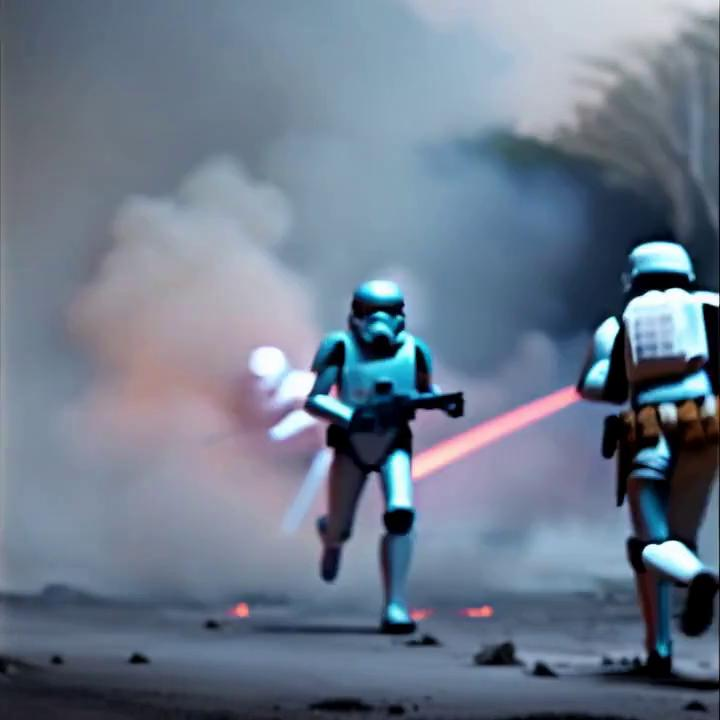}
    \hfill
    \includegraphics[width=0.11\textwidth]{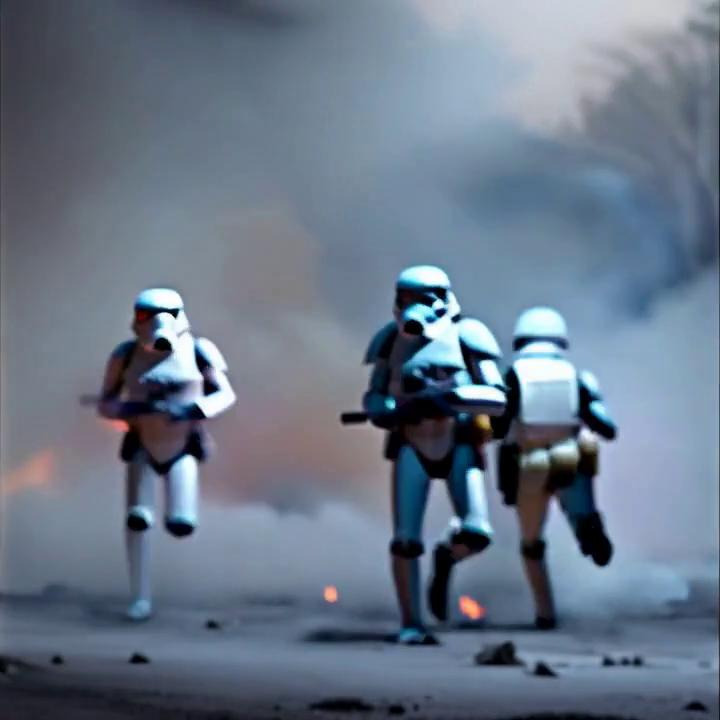}
    \hfill
    \includegraphics[width=0.11\textwidth]{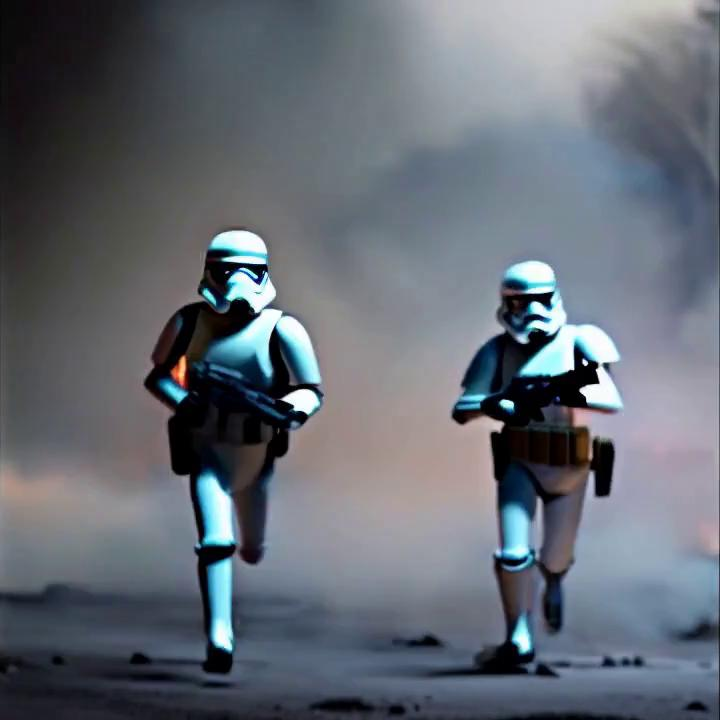}
    \hfill
    \includegraphics[width=0.11\textwidth]{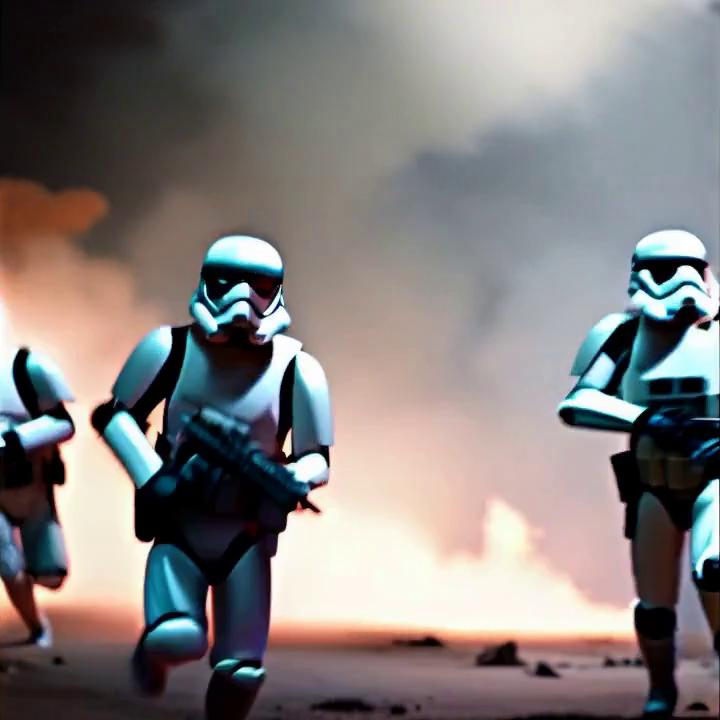}
    \hfill
    \includegraphics[width=0.11\textwidth]{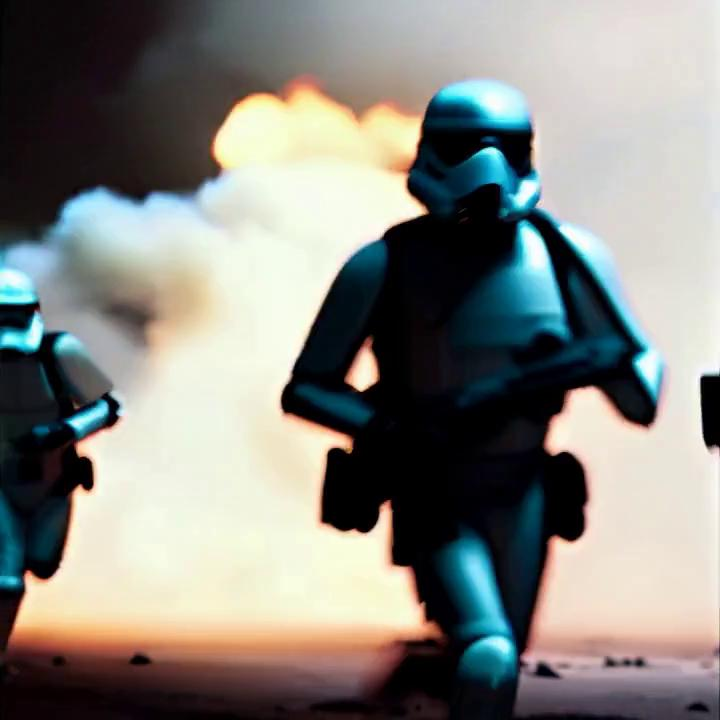}
    \hfill
    \includegraphics[width=0.11\textwidth]{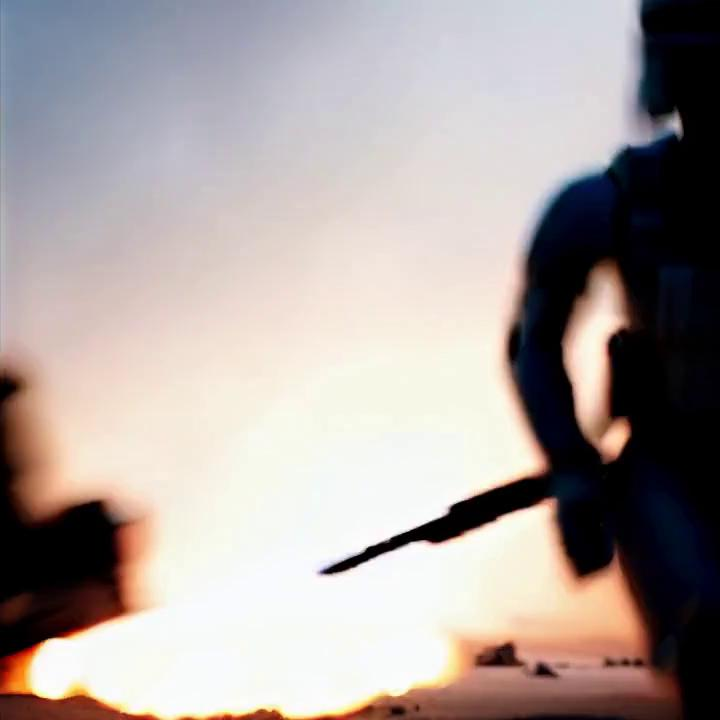}
    \hfill
    \includegraphics[width=0.11\textwidth]{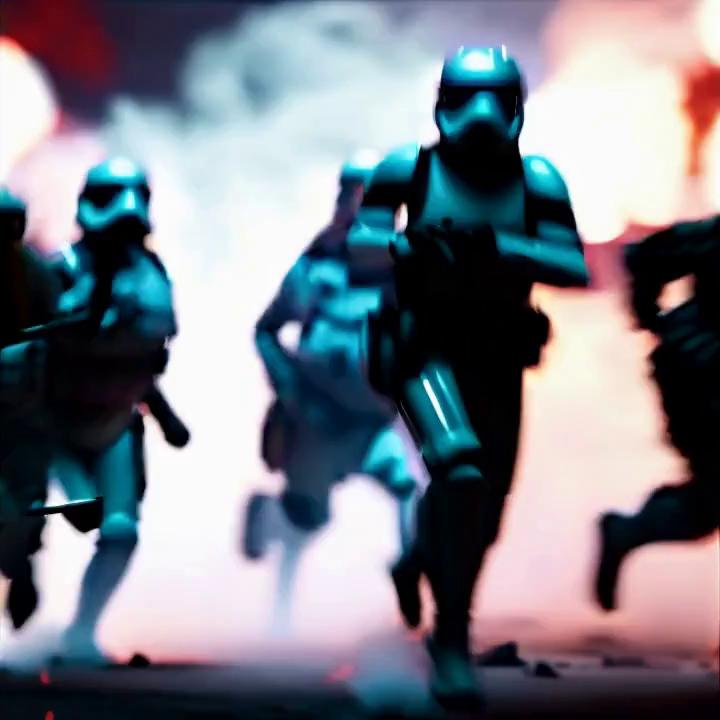}
    \hfill
    
    \caption{Wide shot of battlefield, stormtroopers running at night}
\end{subfigure}

\begin{subfigure}{\textwidth}
    \hspace*{\fill}
    
    \includegraphics[width=0.11\textwidth]{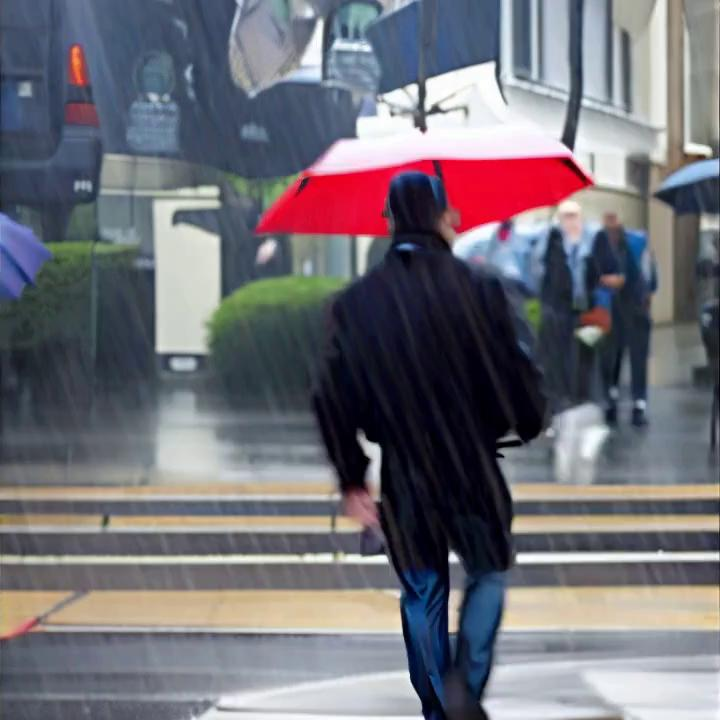}
    \hfill
    \includegraphics[width=0.11\textwidth]{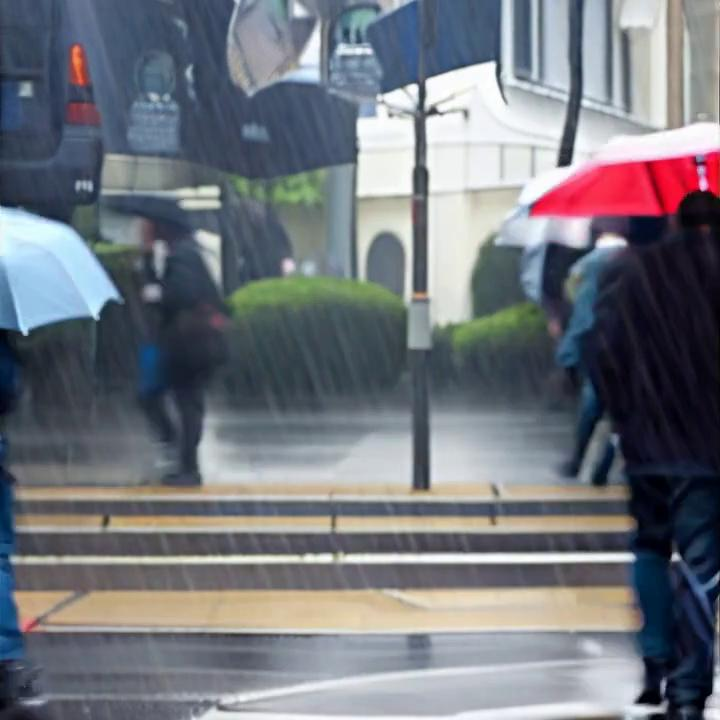}
    \hfill
    \includegraphics[width=0.11\textwidth]{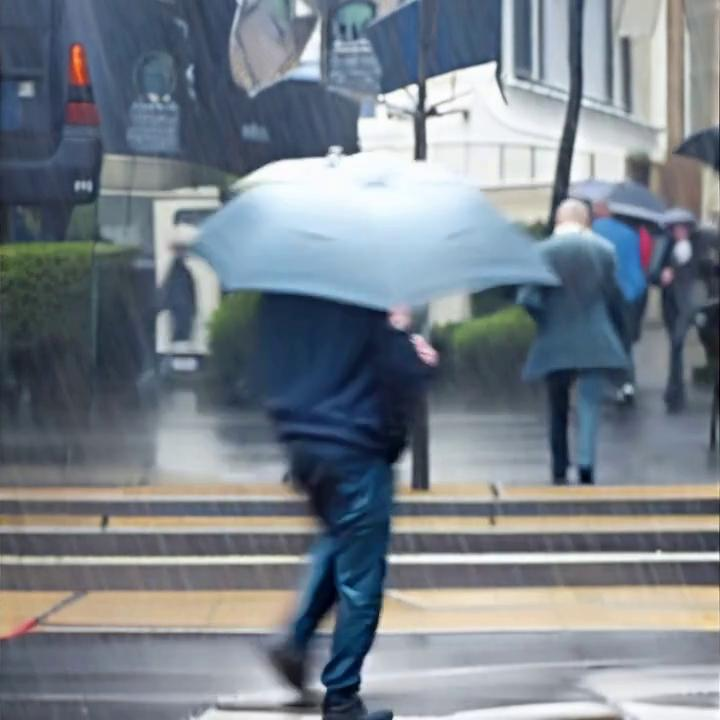}
    \hfill
    \includegraphics[width=0.11\textwidth]{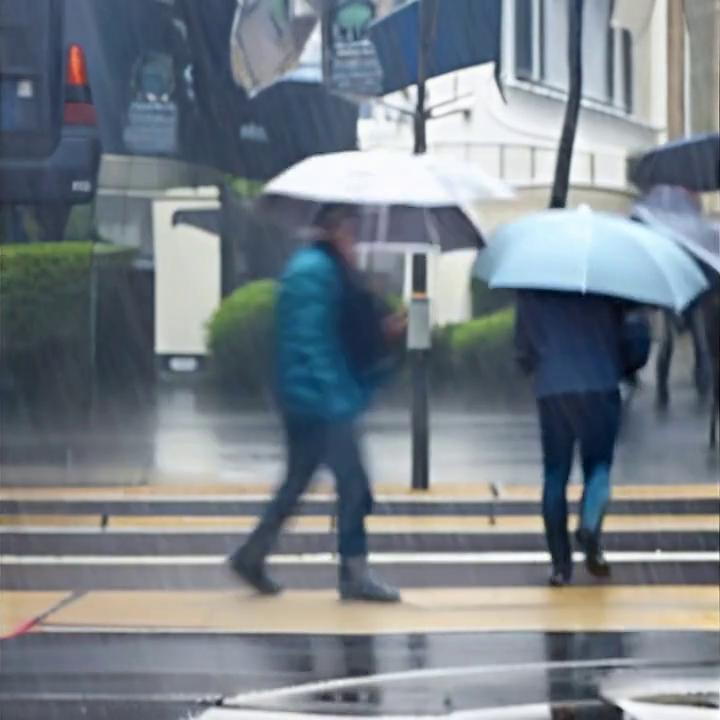}
    \hfill
    \includegraphics[width=0.11\textwidth]{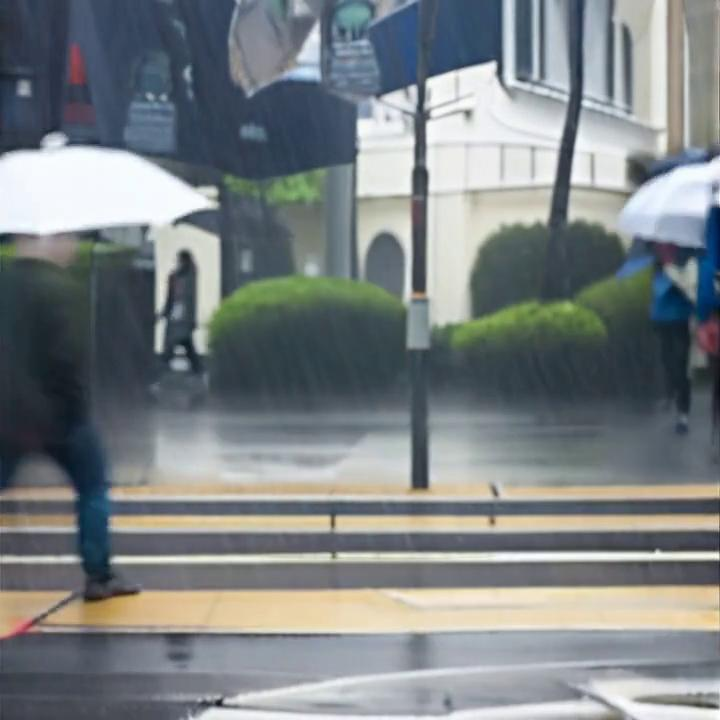}
    \hfill
    \includegraphics[width=0.11\textwidth]{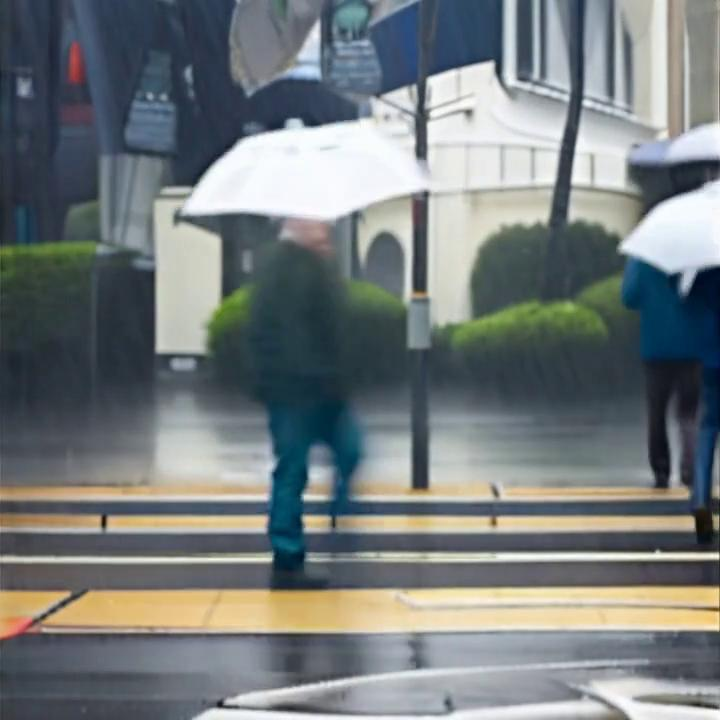}
    \hfill
    \includegraphics[width=0.11\textwidth]{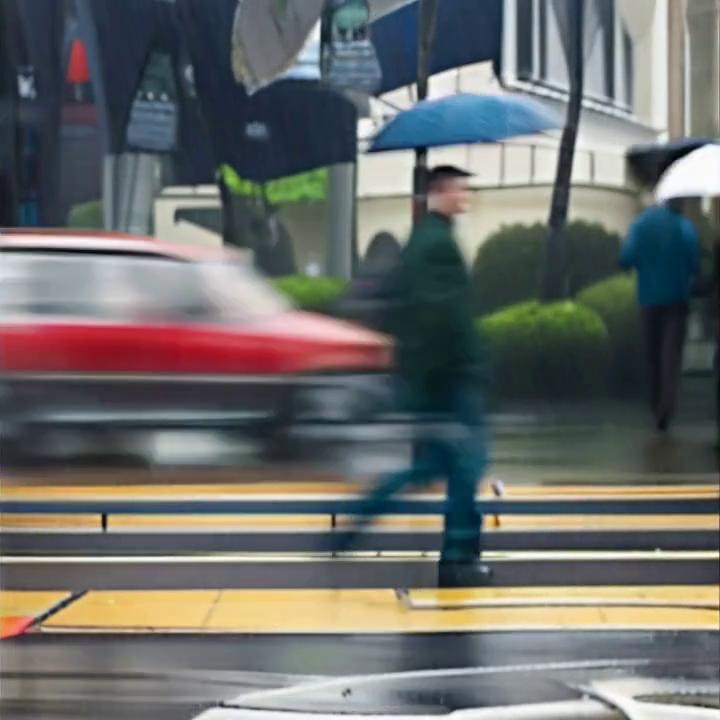}
    \hfill
    \includegraphics[width=0.11\textwidth]{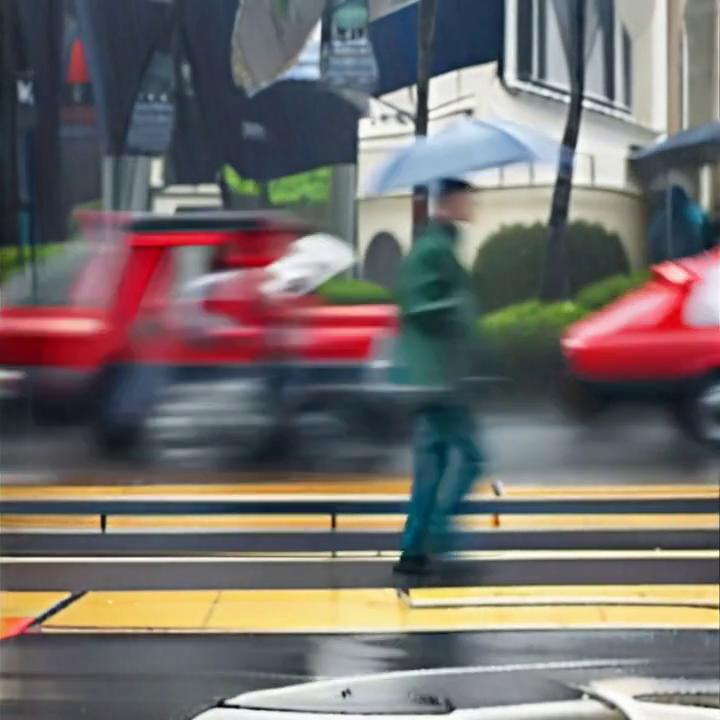}
    \hfill

    \caption{Men walking in the rain}
\end{subfigure}

\begin{subfigure}{\textwidth}
    \hspace*{\fill}
    
    \includegraphics[width=0.11\textwidth]{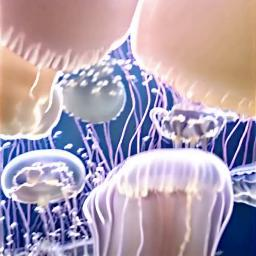}
    \hfill
    \includegraphics[width=0.11\textwidth]{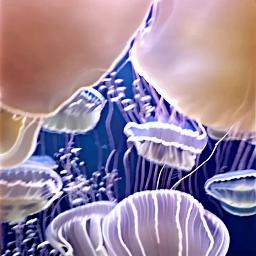}
    \hfill
    \includegraphics[width=0.11\textwidth]{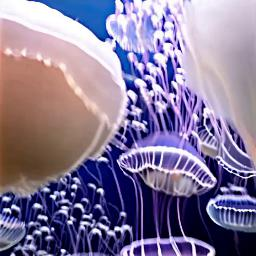}
    \hfill
    \includegraphics[width=0.11\textwidth]{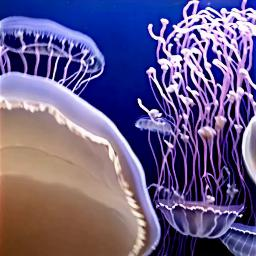}
    \hfill
    \includegraphics[width=0.11\textwidth]{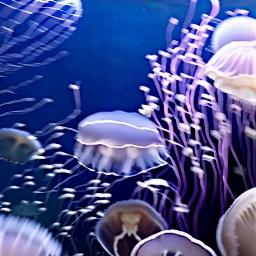}
    \hfill
    \includegraphics[width=0.11\textwidth]{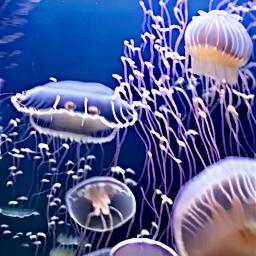}
    \hfill
    \includegraphics[width=0.11\textwidth]{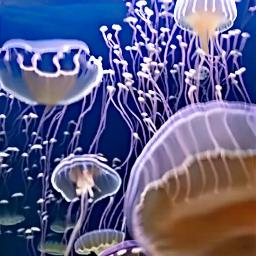}
    \hfill
    \includegraphics[width=0.11\textwidth]{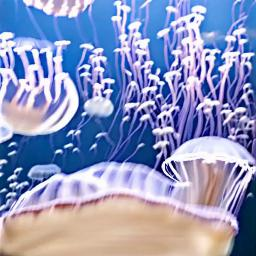}
    \hfill

    \caption{Experience the dance of jellyfish}
\end{subfigure}

\begin{subfigure}{\textwidth}
    \hspace*{\fill}
    
    \includegraphics[width=0.11\textwidth]{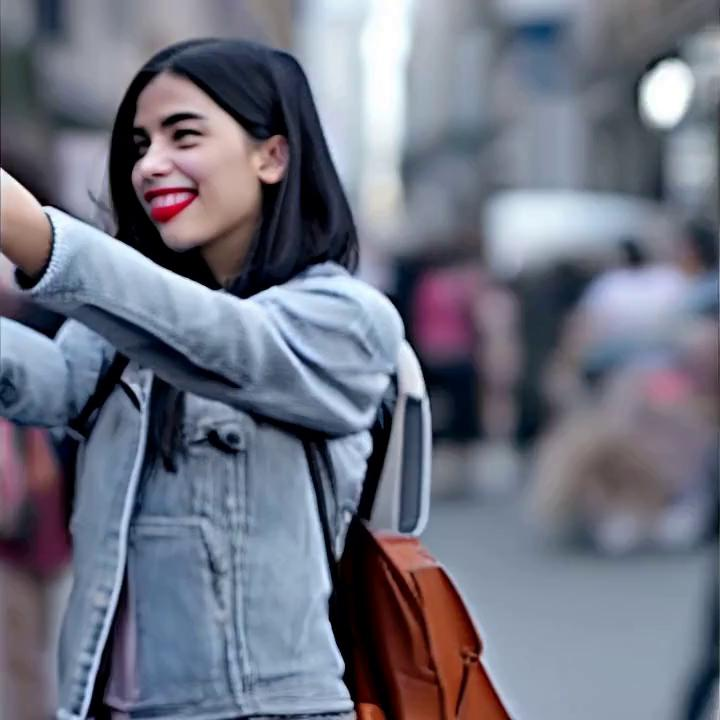}
    \hfill
    \includegraphics[width=0.11\textwidth]{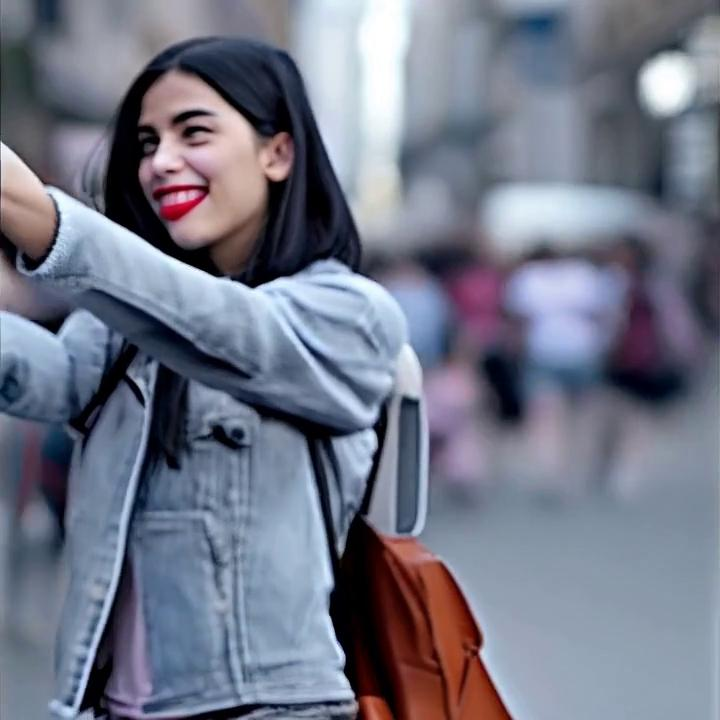}
    \hfill
    \includegraphics[width=0.11\textwidth]{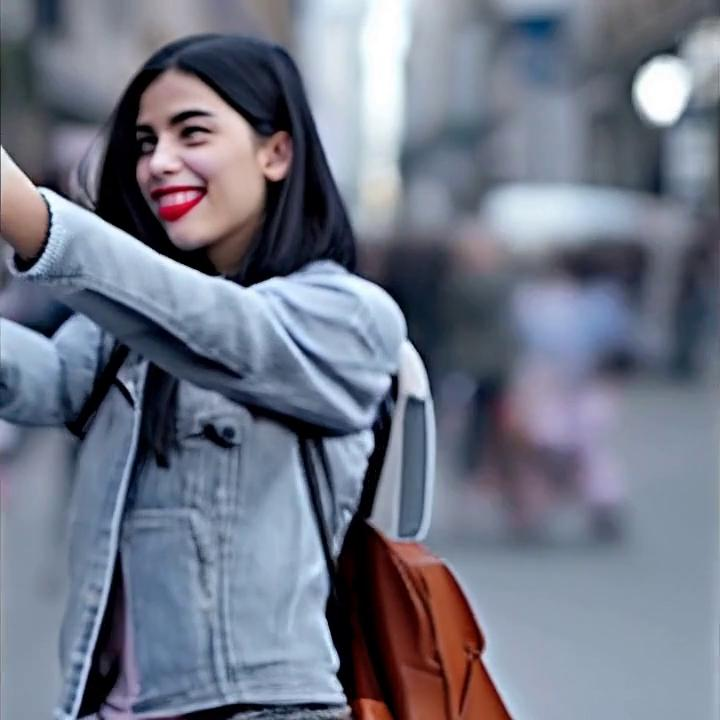}
    \hfill
    \includegraphics[width=0.11\textwidth]{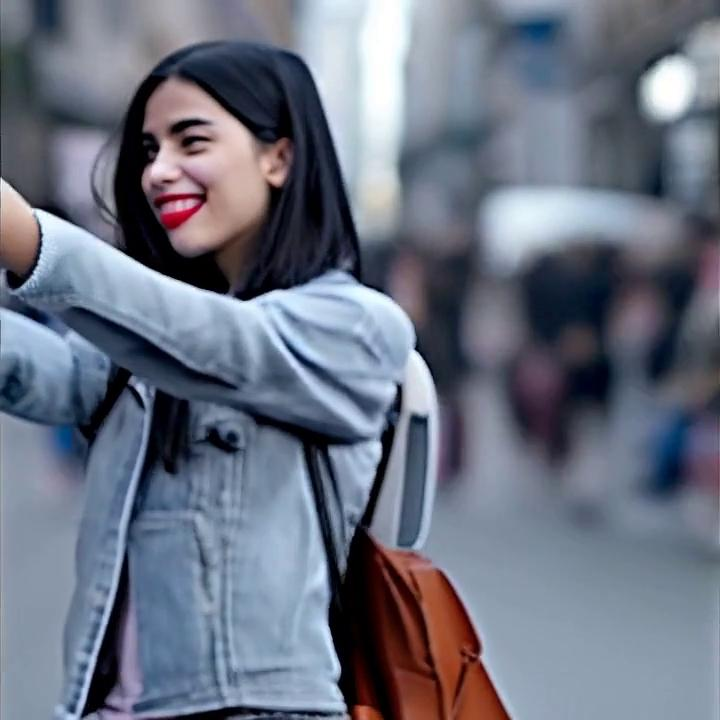}
    \hfill
    \includegraphics[width=0.11\textwidth]{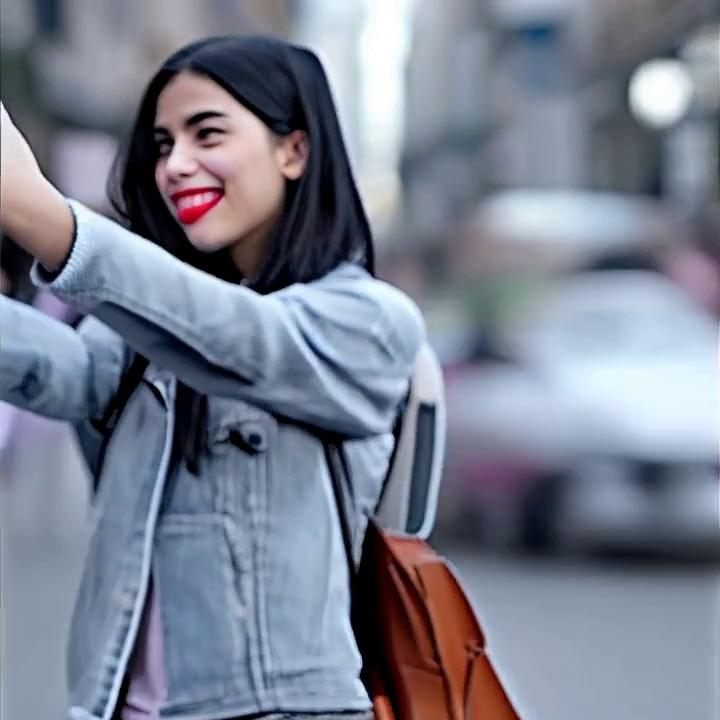}
    \hfill
    \includegraphics[width=0.11\textwidth]{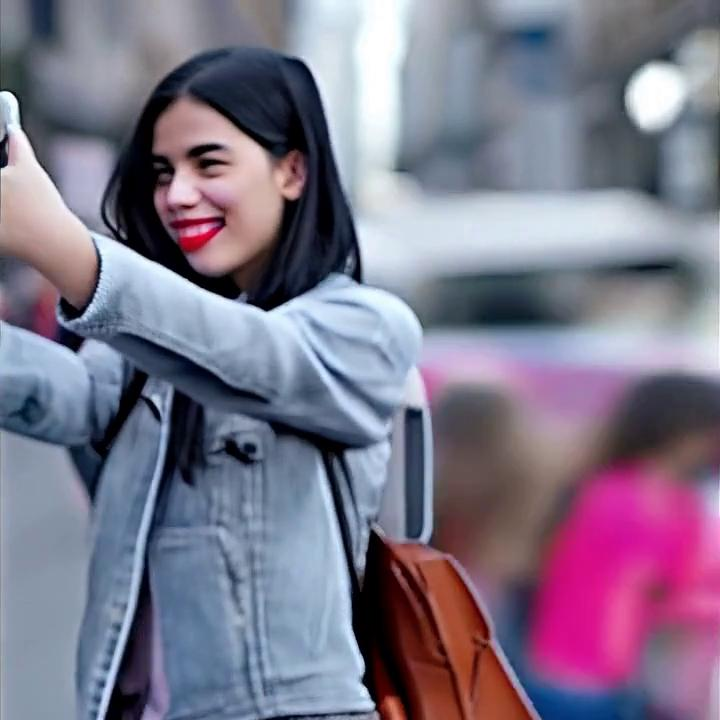}
    \hfill
    \includegraphics[width=0.11\textwidth]{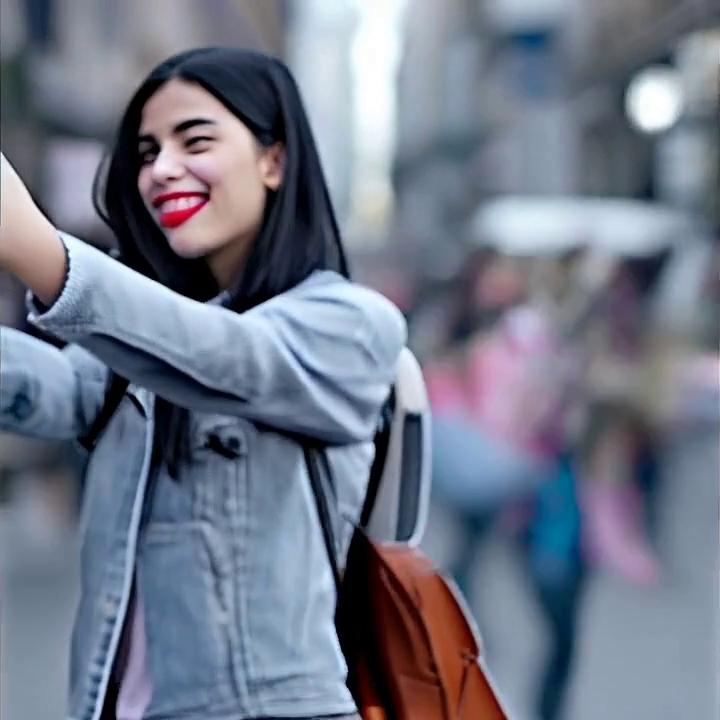}
    \hfill
    \includegraphics[width=0.11\textwidth]{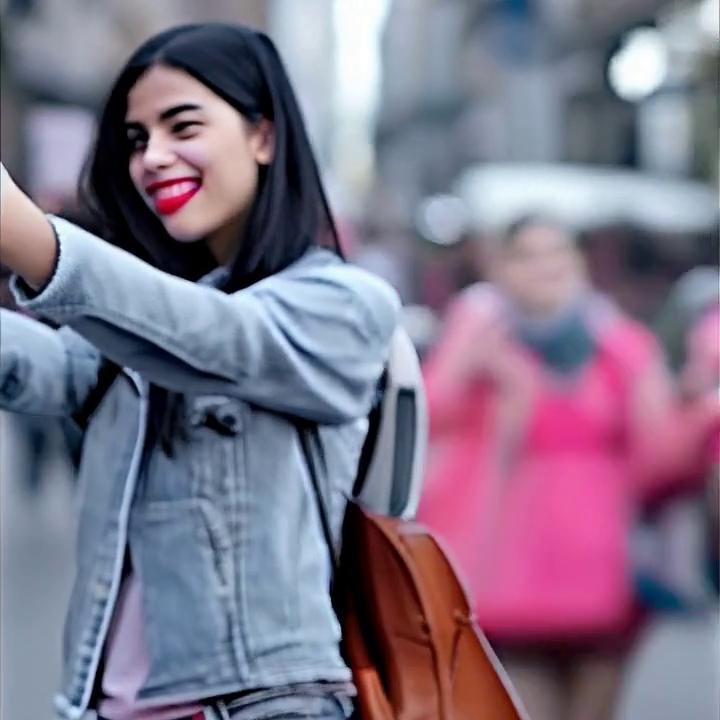}
    \hfill
    
    \caption{A young girl making selfies with her phone in a crowded street}
\end{subfigure}
