# Supplementary material for: StreamingT2V: Consistent, Dynamic, and Extendable Long Video Generation from Text
Source: arXiv:2403.14773 source file (2025-04-16)
Supplement: Supplementary file 3 [file general-2-core.tex]

\begin{tabular}{ m{10.15mm}m{10.15mm}m{10.15mm}m{10.15mm}m{10.15mm}m{10.15mm}m{10.15mm}m{10.15mm}m{10.15mm}m{10.15mm}m{1.1cm}b{0.2cm}}

\includegraphics[width=0.09\textwidth]{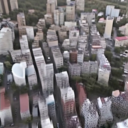}
& \includegraphics[width=0.09\textwidth]{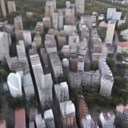}
& \includegraphics[width=0.09\textwidth]{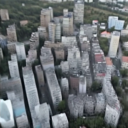}
& \includegraphics[width=0.09\textwidth]{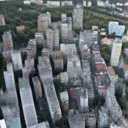}
& \includegraphics[width=0.09\textwidth]{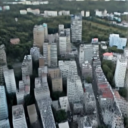}
& \includegraphics[width=0.09\textwidth]{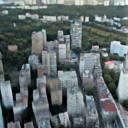}
& \includegraphics[width=0.09\textwidth]{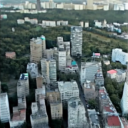}
& \includegraphics[width=0.09\textwidth]{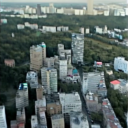}
& \fontsize{6}{12}\selectfont \rotatebox[origin=c]{90}{Ours}
 \\ 

\includegraphics[width=0.09\textwidth]{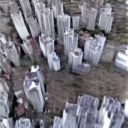}
& \includegraphics[width=0.09\textwidth]{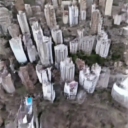}
& \includegraphics[width=0.09\textwidth]{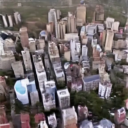}
& \includegraphics[width=0.09\textwidth]{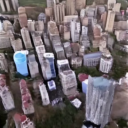}
& \includegraphics[width=0.09\textwidth]{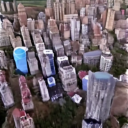}
& \includegraphics[width=0.09\textwidth]{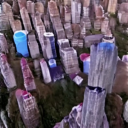}
& \includegraphics[width=0.09\textwidth]{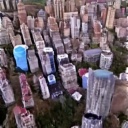}
& \includegraphics[width=0.09\textwidth]{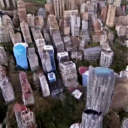}
& \fontsize{6}{12}\selectfont {\rotatebox[origin=c]{90}{\begin{tabular}{@{}c@{}} DC-XL \\ \cite{xing2023dynamicrafter}\end{tabular}}}
 \\ 

\includegraphics[width=0.09\textwidth]{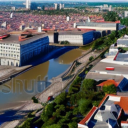}
& \includegraphics[width=0.09\textwidth]{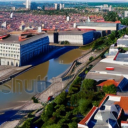}
& \includegraphics[width=0.09\textwidth]{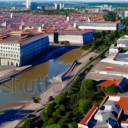}
& \includegraphics[width=0.09\textwidth]{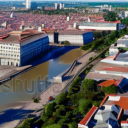}
& \includegraphics[width=0.09\textwidth]{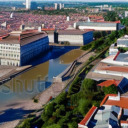}
& \includegraphics[width=0.09\textwidth]{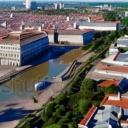}
& \includegraphics[width=0.09\textwidth]{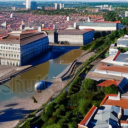}
& \includegraphics[width=0.09\textwidth]{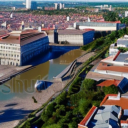}
& \fontsize{6}{12}\selectfont {\rotatebox[origin=c]{90}{\begin{tabular}{@{}c@{}} FreeNse \\ \cite{qiu2023freenoise}\end{tabular}}}
 \\ 

\includegraphics[width=0.09\textwidth]{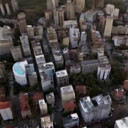}
& \includegraphics[width=0.09\textwidth]{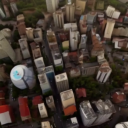}
& \includegraphics[width=0.09\textwidth]{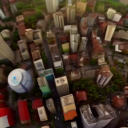}
& \includegraphics[width=0.09\textwidth]{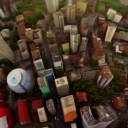}
& \includegraphics[width=0.09\textwidth]{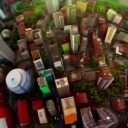}
& \includegraphics[width=0.09\textwidth]{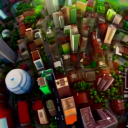}
& \includegraphics[width=0.09\textwidth]{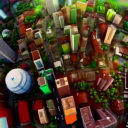}
& \includegraphics[width=0.09\textwidth]{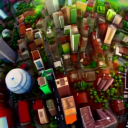}
& \fontsize{6}{12}\selectfont {\rotatebox[origin=c]{90}{\begin{tabular}{@{}c@{}} SpCtrl \\ \cite{guo2023sparsectrl}\end{tabular}}}
 \\ 

\includegraphics[width=0.09\textwidth]{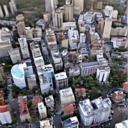}
& \includegraphics[width=0.09\textwidth]{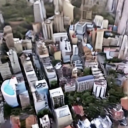}
& \includegraphics[width=0.09\textwidth]{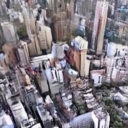}
& \includegraphics[width=0.09\textwidth]{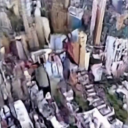}
& \includegraphics[width=0.09\textwidth]{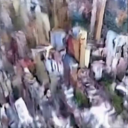}
& \includegraphics[width=0.09\textwidth]{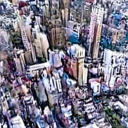}
& \includegraphics[width=0.09\textwidth]{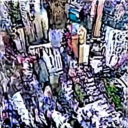}
& \includegraphics[width=0.09\textwidth]{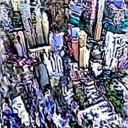}
& \fontsize{6}{12}\selectfont {\rotatebox[origin=c]{90}{\begin{tabular}{@{}c@{}} SVD \\ \cite{SVD}\end{tabular}}}
 \\ 

\includegraphics[width=0.09\textwidth]{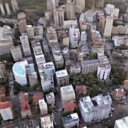}
& \includegraphics[width=0.09\textwidth]{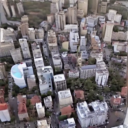}
& \includegraphics[width=0.09\textwidth]{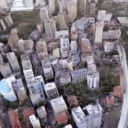}
& \includegraphics[width=0.09\textwidth]{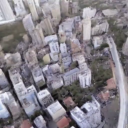}
& \includegraphics[width=0.09\textwidth]{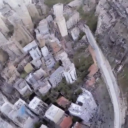}
& \includegraphics[width=0.09\textwidth]{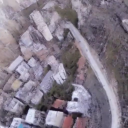}
& \includegraphics[width=0.09\textwidth]{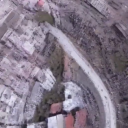}
& \includegraphics[width=0.09\textwidth]{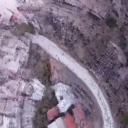}
& \fontsize{6}{12}\selectfont {\rotatebox[origin=c]{90}{\begin{tabular}{@{}c@{}} SEINE \\ \cite{chen2023seine}\end{tabular}}}
 \\ 

\includegraphics[width=0.09\textwidth]{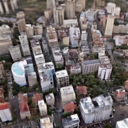}
& \includegraphics[width=0.09\textwidth]{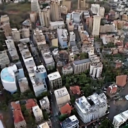}
& \includegraphics[width=0.09\textwidth]{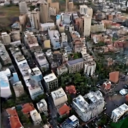}
& \includegraphics[width=0.09\textwidth]{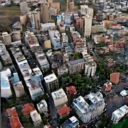}
& \includegraphics[width=0.09\textwidth]{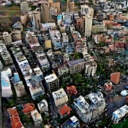}
& \includegraphics[width=0.09\textwidth]{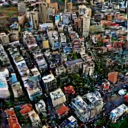}
& \includegraphics[width=0.09\textwidth]{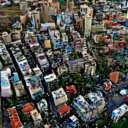}
& \includegraphics[width=0.09\textwidth]{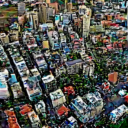}
& \fontsize{6}{12}\selectfont {\rotatebox[origin=c]{90}{\begin{tabular}{@{}c@{}} I2VG \\ \cite{2023i2vgenxl}\end{tabular}}}
 \\ 
\end{tabular}
